# Supplementary material for: Structured Graph Network for Constrained Robot Crowd Navigation with Low Fidelity Simulation
Source: arXiv:2405.16830 source file (2024-05-28)
Supplement: Supplementary file 1 [file Appendix.tex]

\newpage
\section*{Appendix}
\label{sec:append}

\subsection{Limitations and future work}
\label{sec:future}
